# Supplementary material for: Algorithmic complexity of $\beta$-expansions and application to A/D conversion
Source: arXiv:2405.03816 source file (2025-05-27)
Supplement: Supplementary file 1 [file appendices.tex]

% !TEX root = ../main.tex

%%%%%%%%%%%%%%%%%%%%%%%%%%%%%%%%%%%%%%%%%%%%%%%%%%%%%%%%%%%%%%%%%%%%%%%%%%%%%%%%%%%%%%%%%%%%%%%%%%%%
%%%%%%%%%%%%%%%%%%%%%%%%%%%%%%% APPENDIX A %%%%%%%%%%%%%%%%%%%%%%%%%%%%%%%%%%%%%%%%%%%%%%%%%%%%%%%%%
%%%%%%%%%%%%%%%%%%%%%%%%%%%%%%%%%%%%%%%%%%%%%%%%%%%%%%%%%%%%%%%%%%%%%%%%%%%%%%%%%%%%%%%%%%%%%%%%%%%%
%%%%%%%%%%%%%%%%%%%%%%%%%%%%%%%%%%%%%%%%%%%%%%%%%%%%%%%%%%%%%%%%%%%%%%%%%%%%%%%%%%%%%%%%%%%%%%%%%%%%

\section{\texorpdfstring{Definition of $\beta$-expansions by blocks}{}}

The two following results are about computing $\delta_\beta$ when the input is made up of blocks, which turns out to be useful. 
\begin{lemma}\label{lem:factorisation of beta expansion through concatenation}
	Let $n \in \N$, $(\ell_i)_{i \in \ints{0,n}}$, and $(x_i)_{i \in \ints{0,n}} \in \{0,1\}^m$ be a family of $n+1$ binary sequences of respective length $\ell_i$. We define $L_i := \sum_{j=0}^i \ell_j$, for $i \in \ints{0,n}$. Then, for all $\beta \in (1,2]$, it holds that
	\begin{equation}
		\delta_\beta\left(\coprod_{i=0}^n x_i \right) = \delta_\beta(x_0) + \sum_{i=1}^n \beta^{-L_{i-1}} \delta_\beta(x_i).
	\end{equation}
\end{lemma}
\begin{proof} The proof follows by the chain of arguments
	\begin{align}
		\delta_\beta\left(\coprod_{i=0}^n x_i \right) &= \sum_{j=1}^{L_n} \beta^{-j}\left[\coprod_{i=0}^n x_i\right]_j = \sum_{j=1}^{L_0} \beta^{-j}\left[\coprod_{i=0}^n x_i\right]_j + \sum_{j=L_0+1}^{L_n} \beta^{-j}\left[\coprod_{i=0}^n x_i\right]_j\\
		& = \sum_{j=1}^{\ell_0} \beta^{-j}\left[\coprod_{i=0}^n x_0\right]_j + \sum_{j=1}^n \sum_{k=L_{j-1}+1}^{L_j} \beta^{-k}\left[\coprod_{i=0}^n x_i\right]_k\\
		&= \sum_{j=1}^{\ell_0} \beta^{-j}x_0 + \sum_{j=1}^n \sum_{k=1}^{L_j - L_{j-1}} \beta^{-k - L_{j-1}}\left[\coprod_{i=0}^n x_i\right]_{k + L_{j-1}}\\
		&= \delta_\beta(x_0) + \sum_{j=1}^n \beta^{-L_{j-1}}\sum_{k=1}^{\ell_j} \beta^{-k} \left[x_j\right]_k\\
		&= \delta_\beta(x_0) + \sum_{i=1}^n \beta^{-L_{i-1}} \delta_\beta(x_i).
	\end{align}
\end{proof}
\begin{lemma}\label{lem:factorisation of beta expansion through concatenation two}
	Let $x \in \{0,1\}^\ast$ and $\xf \in \{0,1\}^\omega$. Then, for all $\beta \in (1,2]$, it holds that
	\begin{equation}
		\delta_\beta\left( x  \xf \right) = \delta_\beta(x) + \beta^{-|x|} \delta_\beta(\xf).
	\end{equation}
\end{lemma}
\begin{proof}
	The proof follows by the chain of arguments
	\begin{align}
		\delta_\beta\left( x  \xf \right) &=  \sum_{i=1}^\infty [x  \xf]_i\beta^{-i} = \sum_{i=1}^{|x|} [x  \xf]_i\beta^{-i} + \sum_{i=|x| + 1}^{\infty} [x  \xf]_i\beta^{-i}\\
		&= \sum_{i=1}^{|x|} x_i\beta^{-i} + \sum_{i=1}^{\infty} [x  \xf]_{i+|x|}\beta^{-(i+|x|)} =\delta_\beta(x) + \beta^{-|x|} \sum_{i=1}^{\infty} \xf_{i}\beta^{-i}\\
		& =\delta_\beta(x) + \beta^{-|x|} \delta_\beta(\xf).
	\end{align}
\end{proof}

%%%%%%%%%%%%%%%%%%%%%%%%%%%%%%%%%%%%%%%%%%%%%%%%%%%%%%%%%%%%%%%%%%%%%%%%%%%%%%%%%%%%%%%%%%%%%%%%%%%%
%%%%%%%%%%%%%%%%%%%%%%%%%%%%%%% APPENDIX E %%%%%%%%%%%%%%%%%%%%%%%%%%%%%%%%%%%%%%%%%%%%%%%%%%%%%%%%%
%%%%%%%%%%%%%%%%%%%%%%%%%%%%%%%%%%%%%%%%%%%%%%%%%%%%%%%%%%%%%%%%%%%%%%%%%%%%%%%%%%%%%%%%%%%%%%%%%%%%
%%%%%%%%%%%%%%%%%%%%%%%%%%%%%%%%%%%%%%%%%%%%%%%%%%%%%%%%%%%%%%%%%%%%%%%%%%%%%%%%%%%%%%%%%%%%%%%%%%%%

\section{\texorpdfstring{Simple relations for algorithmic complexity of binary and $\beta$-expansions}{Simple relations for algorithmic complexity of binary and -expansions}}
\label{app:greedy binary expansion is a minimizer of Kolmogorov complexity}

\subsection{Proof of Theorem \ref{thm:binary expansion minimizes kolmogorov complexity}}

\begin{lemma}\label{lem:condition prefix beta expansion of x}
	Let $\beta \in (1,2]$, and $s \in \ibet$. Then, for all $x \in \{0,1\}^\ast$, $x$ is a prefix of a $\beta$-expansion if and only if $s \in \delta_\beta(x) +\beta^{-|x|}\left[0,\frac{1}{\beta - 1}\right]$.
\end{lemma}
\begin{proof}
	Let $\beta \in (1,2]$, and $s \in \ibet$. Suppose $s \in \delta_\beta(x) +\beta^{-|x|}\left[0,\frac{1}{\beta - 1}\right]$. Then, there exists $\xf \in \{0,1\}^\omega$ such that
	\begin{equation}
		s = \delta_\beta(x) +\beta^{-|x|}\delta_\beta(\xf) \overset{\ref{lem:factorisation of beta expansion through concatenation two}}{=} \delta_\beta(x  \xf),
	\end{equation}
	so $x$ is a prefix of the $\beta$-expansion $x  \xf$. Conversely, suppose that $x$ is a prefix of a $\beta$-expansion of $s$. Then, there exists $\xf \in \{0,1\}^\omega$ such that $x  \xf$ is a $\beta$-expansion of $s$, i.e.
	\begin{equation}
		s = \delta_\beta(x  \xf)  \overset{\ref{lem:factorisation of beta expansion through concatenation two}}{=} \delta_\beta(x) +\beta^{-|x|}\delta_\beta(\xf) \in \delta_\beta(x) + \beta^{-|x|}\left[0,\frac{1}{\beta - 1}\right].
	\end{equation}
\end{proof}

\begin{lemma}\label{lem:generalization bounding candidates greedy expansion}
	Let $\beta_1,\beta_2 \in (1,2), \ \beta_1 < \beta_2$, $n \in \N$ and $x \in \{0,1\}^n$. We denote by $A(x)$ the set of $\lceil n \log_2(\beta_1)\rceil$-prefixes of the greedy expansions of all real numbers for which there exists $\beta \in (\beta_1,\beta_2)$ such that one of the $\beta$-expansions has $n$-prefix $x$. Then,
	\begin{equation}
		\#\left(A(x)\right) \leq \frac{2}{\beta_1 - 1} + n(n+1)(\beta_2 - \beta_1)\beta_1^{n} + 2.
	\end{equation}
\end{lemma}
\begin{proof}
	Let $\beta_1,\beta_2 \in (1,2], \ \beta_1 < \beta_2$, $n \in \N$ and $x \in \{0,1\}^n$. Let $X(x) \subseteq \left[0, \frac{1}{\beta_1 - 1}\right)$ be the set of real numbers for which there exists $\beta \in (\beta_1,\beta_2)$ such that one of the $\beta$-expansions has prefix $x$. By Lemma \ref{lem:condition prefix beta expansion of x}, 
	\begin{equation}
		S(x) = \bigcup_{\beta \in [\beta_1,\beta_2]} \left(\delta_\beta(x) + \beta^{-n}\left[0,\frac{1}{\beta - 1}\right]\right).
	\end{equation}
	Note that $t \mapsto \delta_t(b)$, as a function from $(1,2]$ to $\R$, is continuous and decreasing, so $S(x)$ is a closed interval whose lower bound is $\delta_{\beta_2}(x)$ and $\delta_{\beta_1}(x) + \frac{\beta_1^{-n}}{\beta_1-1}$ is the upper bound, i.e.
	\begin{equation}
		S(x) = \left[\delta_{\beta_2}(x),\delta_{\beta_1}(x) + \frac{\beta_1^{-n}}{\beta_1 - 1}\right].
	\end{equation}
	Let $w \in \{0,1\}^{\lceil n \log_2(\beta_2)\rceil}$. One has that $y \in A(x)$ $\Leftrightarrow$ there exists a $s \in S(x)$ such that $y$ is a prefix of $\gf_2(s)$ $\overset{\ref{lem:condition prefix beta expansion of x}}{\Rightarrow}$ there exists $s \in X(x)$ such that $s \in \delta_2(y) + 2^{-|y|}\left[0,1\right]$ $\Leftrightarrow$ there exists $s \in S(x)$ such that $\delta_2(y) \in s + 2^{-|y|}\left[-1, 0\right]$ $\Leftrightarrow$ $\delta_2(y) \in S(x) + 2^{-|y|}\left[-1, 0\right] = \left[\delta_{\beta_2}(x)- 2^{-|y|},\delta_{\beta_1}(x) + \frac{\beta_1^{-n}}{\beta_1 - 1}\right]$. Therefore,
	\begin{equation}
		A(x) \subseteq \delta_2\left(\{0,1\}^{\lceil n \log_2(\beta_1)\rceil}\right) \cap \underset{=: R(x)}{\underbrace{\left[\delta_{\beta_2}(x)- 2^{-|y|},\delta_{\beta_1}(x) + \frac{\beta_1^{-n}}{\beta_1 - 1}\right]}}.
	\end{equation}
	As for any two different elements of $s,s' \in \delta_2\left(\{0,1\}^{\lceil n \log_2(\beta_1)\rceil}\right)$, $|s - s'| \geq d := 2^{-\lceil n \log_2(\beta_1)\rceil}$, one has
	\begin{align}
		\#(A(x)) &\leq \left\lceil \frac{|R(x)|}{d}\right\rceil \leq \frac{\left[\delta_{\beta_2}(x)- 2^{-\lceil n \log_2(\beta_1)\rceil},\delta_{\beta_1}(x) + \frac{\beta_1^{-n}}{\beta_1 - 1}\right]}{2^{-\lceil n \log_2(\beta_1)\rceil}} + 1\\
		&= \frac{2^{-\lceil n \log_2(\beta_1)\rceil} + \frac{\beta_1^{-n}}{\beta_1 - 1} + \delta_{\beta_1}(x) - \delta_{\beta_2}(x)}{2^{-\lceil n \log_2(\beta_1)\rceil}} + 1\\
		& = \frac{2^{-\lceil n \log_2(\beta_1)\rceil}\beta_1^{-n}}{\beta_1 - 1} + 2^{-\lceil n \log_2(\beta_1)\rceil} \left(\delta_{\beta_1}(x) - \delta_{\beta_2}(x)\right) + 2 \\
		&\leq \frac{2^{-n \log_2(\beta_1) + 1}\beta_1^{-n}}{\beta_1 - 1} + 2^{-n \log_2(\beta_1) + 1} \left(\delta_{\beta_1}(x) - \delta_{\beta_2}(x)\right) + 2\\
		 &\leq \frac{2}{\beta_1 -1} + 2\beta_1^n \left(\delta_{\beta_1}(x) - \delta_{\beta_2}(x)\right) + 2\\
		 &\leq \frac{2}{\beta_1 -1} + 2\beta_1^n \frac{n(n+1)}{2} (\beta_2-\beta_1) + 2\\
		 &= \frac{2}{\beta_1 -1} + \beta_1^n n(n+1) (\beta_2-\beta_1) + 2.
	\end{align}
\end{proof}

\begin{theorem}\label{lemma:generalized app beta expansions are more complex than the binary expansion}
	For all $s \in [0,1]$ and all $\beta \in (1,2)$, there exists $c > 0$ such that
\begin{equation}
	K[\gf_2(s)|\lceil n \log_2(\beta)\rceil] \leq K[\xf|n] + F(K[u_n]) + c, \ \ \forall n \in \N, \ \ \forall \xf \in \Sigma_\beta(s),
\end{equation}
where $u_n := \gf_2(\beta-1)_{1: n}$, and $F: t \mapsto t + 2\log_2(t)$.
\end{theorem}
\begin{proof}
The main arguments of this proof follow closely that of \cite[Theorem 3]{staiger2002kolmogorov}. Let $s \in [0,1]$, $\beta \in (1,2)$, $\xf \in \Sigma_\beta(s)$ and $n \in \N$, large enough to ensure that $u_n := \gf_2(\beta - 1)_{1: n}$ is not made only of $0$'s. Let $\beta_1 - 1 \in (0,1)\cap \Q$ to be the real number having the same greedy binary expansion as $\beta - 1$, but truncated after $\lceil n \log_2(\beta)\rceil$ bits, i.e. $\beta_1 - 1 := \delta_2(u_n)$.
We also define $\beta_2 := \beta_1 + 2^{-\lceil \log_2(\beta)\rceil}$. By Lemma \ref{lem:condition prefix beta expansion of x}, 
\begin{equation}
	1 \overset{(a)}{<} \beta_1 \leq \beta \leq \beta_2 \leq 2.
\end{equation}
where (a) follows from the fact that $u_n$ is not made only of $0$'s.

By Lemma \ref{lem:generalization bounding candidates greedy expansion}, the sole knowledge of $\xf_{1: n}$ allows to immediatly conclude that $\gf_2(s)_{1: \lceil n \log_2(\beta) \rceil}$ belongs to a set $A(\xf_{1: n}) \subseteq \{0,1\}^{\lceil n \log_2(\beta_1) \rceil}$, which cardinality is bounded above by $\frac{2}{\beta_1 - 1} + n(n+1)(\beta_2 - \beta_1)\beta_1^{n} + 2$, and which can be computed by using $u_n$ only. As defined above, $\beta_2 - \beta_1 = 2^{-\lceil \log_2(\beta)\rceil} \leq \beta^{-n}$, hence $n(n+1)(\beta_2 - \beta_1)\beta_1^n \leq n(n+1) (\beta_1/\beta)^n$. As $\beta_1/\beta < 1$, $\left(n(n+1) (\beta_1/\beta)^n\right)_{n \in \N}$ is a bounded sequence. Overall, there exists a constant $N > 0$, independant of $n$, such that $\#(A(\xf_{1: n})) \leq N$.

Let $z_n \in \N$ be the index of $\gf_2(s)_{1: \lceil n \log_2(\beta) \rceil}$ in the lexicographical enumeration of $A(\xf_{1: n})$. Then, one can build an effective algorithm $\varphi : \{0,1\}^\ast \to \{0,1\}^\ast$, such that on input $\langle \langle\xf_{1: n}, u_n \rangle,  z_n \rangle$, $\varphi$ computes $A(\xf_{1: n})$, finds the $z_n$-th element $y$ of $A(\xf_{1: n})$ and outputs $y$.
 By the preceding discussion, it is clear that $\varphi(\langle \langle \xf_{1: n},  u_n\rangle,  z_n  \rangle) = \gf_2(s)_{1: \lceil n \log_2(\beta) \rceil}$. By Lemma \ref{lem:if two sequences are connected through an algorithm, they have same kolmogorov complexity}, there exists $C,C' > 0$ such that 
 \begin{align}\label{eq:first bounding of kolmogorov complexity of greedy binary expansion}
	K[y] &\overset{\ref{lem:if two sequences are connected through an algorithm, they have same kolmogorov complexity}}{\leq} K[\langle \langle\xf_{1: n}, z_n \rangle,  u_n \rangle ] + C\\
	&\overset{(\ref{eq:simple inequality on concatenation of sequences})}{\leq} K[\langle \xf_{1: n}, z_n \rangle] + F\left(K[u_n]\right) + C_+ + C\\
	&\overset{(\ref{eq:simple inequality on concatenation of sequences})}{\leq} K[\xf_{1: n}] + F\left(K[z_n]\right) + F\left(K[u_n]\right) + 2C_+ + C\\
	&\overset{(\ref{eq:algorithmic complexity is bounded by the length})}{\leq} K[\xf_{1: n}] + F\left(|z_n|+ C_{||}\right) + F\left(K[u_n]\right) + 2C_+ + C\\
	&\overset{\ref{lem:if two sequences are connected through an algorithm, they have same kolmogorov complexity}}{\leq} K[\xf_{1: n}] + F\left(|z_n|+ C_{||}\right) + F\left(K[u_n] + C'\right)  + 2C_+ + C\\
	&\overset{(a)}{\leq} K[\xf_{1: n}] + F\left(|z_n|\right) + F\left(K[u_n]\right) + C_{||} + 2C_+ + C + C',\label{eq:ineq algorithmic complexity w appendix}
 \end{align}
 where $(a)$ is by $F$ being subadditive.
 Recall from above that $\#(A(\xf_{1:n})) \leq N$. As $z_n$ is an index for $A(\xf_{1:n})$, then $z_n \leq N$, and we set $C_0 :=  F(N)$, so that 
 \begin{equation}
 K[y] \overset{(\ref{eq:ineq algorithmic complexity w appendix})}{\leq} K[\xf_{1: n}] + F\left(K[u_n]\right) + C_{||} + 2C_+ + C + C' + C_0.
 \end{equation}
We set $c := C_{||} + 2C_+ + C + C' + C_0$. By identification of $y$ with $\gf_2(s)_{1: \lceil n \log_2(\beta_1) \rceil}$, one has 
 \begin{equation}\label{eq:almost the end of the proof}
		K[\gf_2(s)|\lceil n \log_2(\beta_1) \rceil] \leq K[\xf|n] + F(K[u_n]) + c.
 \end{equation}
 Note that as $\beta_1 := \delta_2(u_n)$, $|\beta - \beta_1| \leq 2^{-\lceil n \log_2(\beta)\rceil} \leq \beta^{-n}$, so
 \begin{align}
	\left|\lceil n \log_2(\beta) \rceil - \lceil n \log_2(\beta_1) \rceil\right| & \leq n (\log_2(\beta) - \log_2(\beta_1)) + 2\\
	& = n (\log_2(\beta_1 + \beta^{-n}) - \log_2(\beta_1)) + 2\\
	& = n (\log_2(1 + \beta_1^{-1}\beta^{-n})) + 2 \\
	&\leq n \beta_1^{-1}\beta^{-n} + 2\\
	&\overset{(a)}{\leq} \frac{\beta_1^{-1}}{\log(\beta)}\beta^{-\frac{1}{\log(\beta)}} + 2 =: D,
 \end{align}
 where is a consequence of a study of the maximum of the functiono $t \mapsto t\beta^{-t}$. By application of Lemma \ref{lem:kolmogorov complexity of closed sequences}, there exists $D' > 0$ such that
 \begin{equation}\label{eq:comparable kolmogorov complexities for approximations}
	K[\gf_2(s)|\lceil n \log_2(\beta) \rceil] \leq K[\gf_2(s)|\lceil n \log_2(\beta_1) \rceil] + D'.
 \end{equation}
By (\ref{eq:almost the end of the proof}) and (\ref{eq:comparable kolmogorov complexities for approximations}), one gets
\begin{equation}
	K[\gf_2(s)|\lceil n \log_2(\beta) \rceil] \leq K[\xf|n] + F(K[u_n]) + c + D',
\end{equation}
thereby finishing the proof.
\end{proof}

\subsection{Proof of Theorem \ref{thm:upper bound kolmogorov complexity beta expansions}}

\textit{To appear.}

\section{Miscellaneous results}

\begin{lemma}
	\cite[Example 2.1.5]{li2008introduction} There exists $C_+>0$, such that
	\begin{align}\label{eq:simple inequality on concatenation of sequences}
		K[ x x'] &\leq K[x] + F(K[x']) + C_+, \ \ \text{for all} \ x,x' \in \{0,1\}^\ast,
	\end{align}
	and
	\begin{align}\label{eq:simple inequality on pairing of sequences}
		K[ \langle x, x'\rangle] &\leq K[x] + F(K[x']) + C_+, \ \ \text{for all} \ x,x' \in \{0,1\}^\ast,
	\end{align}
	where $F:t\mapsto t + 2\log_2(t)$.
\end{lemma}
\begin{lemma}\cite[Theorem 2.1.2]{li2008introduction} There exists $C_{||} > 0$, such that 
	\begin{equation}\label{eq:algorithmic complexity is bounded by the length}
		K[x] \leq |x| + C_{||}, \ \ \text{for all} \ x \in \{0,1\}^\ast.
	\end{equation}
\end{lemma}
\begin{lemma}
	Let $N \in \N$, $\xf \in \{0,1\}^\omega$, $(u_n)_{n \in \N}$ a sequence of integers. Then, 
	\begin{equation}
		K[\xf|N n] \leq u_n, \ \forall n \in \N \Rightarrow \exists C > 0 \ s.t. \ K[\xf|n] \leq u_{\lfloor n/N \rfloor } + C, \ \forall n \in \N.
	\end{equation}
\end{lemma}
\begin{proof}
	Let $N \in \N$, $\xf \in \{0,1\}^\omega$, $(u_n)_{n \in \N}$ a sequence of integers, and suppose that $K[\xf|N n] \leq u_n, \ \forall n \in \N$. Fix $n \in \N$. Then, $k := \lfloor n/N \rfloor$ satisfies $n = kN + (n - kN)$, where $n - kN \leq N$. Then,
	\begin{align}
		K[\xf|n] &= K[\xf_{1: n}] = K[\xf_{1: kN}  \xf_{1: (n- kN)}] \\
		&\overset{(\ref{eq:simple inequality on concatenation of sequences})}{\leq} K[\xf_{1: kN}] + K[\xf_{1: (n- kN)}] + 2 \log_2 (K[\xf_{1: (n- kN)}]) + C_+\\
		&\overset{(a)}{\leq} K[\xf_{1: kN}] + N + C_{||} + 2 \log_2 (N + C_{||}) + C_{+}\\
		&\overset{(b)}{\leq} u_k + N + C_{||} + 2 \log_2 (N + C_{||}) + C_{+}\\
		&= u_{\lfloor n/N \rfloor} + N + C_{||} + 2 \log_2 (N + C_{||}) + C_{+},
	\end{align}
	where (a) follows from (\ref{eq:algorithmic complexity is bounded by the length}) and $n - kN \leq N$, and (b) is by $K[\xf|N k] \leq u_k$. We set $C:= N + C_{||} + 2 \log_2 (N + C_{||}) + C_{+}$, thereby finishing the proof.
\end{proof}
\begin{lemma}\label{lem:kolmogorov complexity of closed sequences}
	Let $\xf \in \{0,1\}^\omega$, $(i_n)_{n \in \N}$ and $(j_n)$ be two increasing sequences of natural numbers. Suppose that there exists $M > 0$ such that $|i_n-j_n| \leq M$, for all $n \in \N$. Then, there exists $C>0$, such that
	\begin{equation}
		K[\xf|i_n] \leq K[\xf|j_n] + C, \ \text{for all} \ n \in \N.
	\end{equation}
\end{lemma}
\begin{proof}
	Let $\xf \in \{0,1\}^\omega$, $(i_n)_{n \in \N}$ and $(j_n)$ be two increasing sequences of natural numbers. Suppose that there exists $M > 0$ such that $ |i_n-j_n| \leq M$, for all $n \in \N$. Fix $n \in \N$, and let $x:= 10^{j_n + M-i_n}$. Then, one can build an effective algorithm $\phi: \{0,1\}^\ast \to \{0,1\}^\ast$, which on input $\xf_{1: j_n + M}  x$, which uses $x$ to delete the $j_n + M - i_n$ last bits of $\xf_{1: j_n + M}$, and outputs the resulting sequence. Then, $\phi(\xf_{1: j_n + M}  x) = \phi(\xf_{1: i_n})$. By Lemma \ref{lem:if two sequences are connected through an algorithm, they have same kolmogorov complexity}, there exists $c_\phi > 0$ such that
	\begin{align}
		K[\xf|i_n] &= K[\xf_{1: i_n}] \leq K[\xf_{1: j_n}  x] + c_\phi\\
		&\overset{(\ref{eq:simple inequality on concatenation of sequences})}{\leq} K[\xf_{1: j_n}] + K[x] + 2\log(K[x]) +c_{\phi} + C_{+}\\
		&\overset{(\ref{eq:algorithmic complexity is bounded by the length})}{\leq} K[\xf_{1: j_n}] + |x| + C_{||} + 2 \log_2 (|x| + C_{||}) + c_\phi + C_{+}\\
		&\overset{(a)}{\leq} K[\xf_{1: j_n}] + 2M + C_{||} + 2 \log_2 (2M + C_{||}) + c_\phi + C_{+},
	\end{align}
	where (a) is by $|x| = j_n + M - i_n$ and $i_n - M \leq j_n$. We set $C:= 2M + C_{||} + 2 \log_2 (2M + C_{||}) + c_\phi+ C_{+}$, thereby finishing the proof.
\end{proof}
